# Supplementary material for: Streaming Algorithms for Ellipsoidal Approximation of Convex Polytopes
Source: arXiv:2206.07250 source file (2022-06-15)
Supplement: Supplementary file 2 [file appendix_online_coreset.tex]

\section{Subspace Sketching}
\label{sec:subspace_sketching}

In this section, we describe an extension of our techniques to the setting studied in \cite{woodruff2022high}.

First, we restate the main problem studied in \cite{woodruff2022high}.

\begin{problem}[Streaming $\linf$ subspace sketching -- See Definition 1.1 of \cite{woodruff2022high}]
\label{problem:subspace_sketching}
In what follows, for a matrix $X \in \R^{n\times d}$ and a subset $S \subseteq [n]$, let $X\vert_S$ be the matrix obtained by restricting $X$ to the rows indexed by $S$.

Let $X \in \R^{n\times d}$ be a matrix given to us in a row arrival stream. Then:
\begin{itemize}
    \item In the \emph{row arrival streaming model}, let $X \in \Z^{n\times d}$ have entries bounded by $\mathsf{poly}(n)$. We must maintain a data structure $\myfunc{Q}{\R^d}{\R}$ such that, at the end of the stream, we have for some $\alpha \ge 1$ that:
    \begin{align*}
        \text{for all } y \in \R^d, \maxnorm{Xy} \le Q(y) \le \alpha \cdot \maxnorm{Xy}
    \end{align*}
    \item In the \emph{online coreset model}, let $X \in \R^{n \times d}$ be a real matrix. We must irrevocably choose a subset of entries $S \subseteq [n]$ and weights $w \in \R^S$ as well as a function $\myfunc{Q}{\R^d}{\R}$ depending only on $\diag{w}X\vert_S$ such that, at the end of the stream, we have for some $\alpha \ge 1$ that:
    \begin{align*}
        \text{for all } x \in \R^d, \maxnorm{Xy} \le Q(y) \le \alpha \cdot \maxnorm{Xy}
    \end{align*}
\end{itemize}
\end{problem}

The authors of \cite{woodruff2022high} give algorithmic results for Problem \ref{problem:subspace_sketching} (see Theorem \ref{thm:subspace_sketching}). They use this as a meta-approach to give algorithms for a variety of streaming linear algebra and streaming computational geometry tasks, including convex hull sketching, streaming ellipsoidal approximations\footnote{The approximation factor given in \cite{woodruff2022high} for streaming ellipsoidal approximations is suboptimal by a factor of $\Omega\inparen{\sqrt{d}}$; see Theorem 1.10.}, $k$-robust directional width, $\ell_p$ subspace sketch for $p < \infty$, volume maximization, minimum-width spherical shell, and solving linear programs. See Section 1.1 of \cite{woodruff2022high} for more details.

\begin{theorem}[See Theorem 1.3 of \cite{woodruff2022high}]
\label{thm:subspace_sketching}
Let $\kappaol$ be the \emph{online condition number} of $X$ -- that is, $\kappaol(X) \coloneqq \opnorm{X} \cdot \max_{i \in [n]} \opnorm{X\vert_{[i]}^{+}}$, where $X^{+}$ denotes the Moore-Penrose pseudoinverse of $X$.

Let $X \in \R^{n \times d}$ be presented in one pass over a row arrival stream. There is an algorithm $\cA$ which maintains a coreset $S \subseteq [n]$ such that:
\begin{align*}
    \text{for all } y \in \R^d, \maxnorm{X\vert_S \cdot y} \le \maxnorm{Xy} \le \alpha \cdot \maxnorm{X\vert_S \cdot y}
\end{align*}
where:
\begin{itemize}
    \item in the row arrival streaming model, $\alpha = O\inparen{\sqrt{d \log n}}$, $\abs{S} = O(d \log n)$, and $\cA$ uses $O(d^2 \log^2 n)$ bits of space.
    \item in the online coreset model, $\alpha = O\inparen{\sqrt{d\log \kappaol(X)}}$ and $\abs{S} = O\inparen{d \log \kappaol(X)}$.
\end{itemize}
\end{theorem}

The authors of \cite{woodruff2022high} use a simple greedy algorithm to witness Theorem \ref{thm:subspace_sketching}. To analyze this algorithm, they bound the sum of \emph{online ridge leverage scores}.

In the remainder of this section, we recover a result similar to that of Theorem \ref{thm:subspace_sketching} using the update rule from Algorithm \ref{alg:greedy_maxev}. See Algorithm \ref{alg:subspace_sketching} (in an abuse of notation, let $X\vert_S = \conv{\inbraces{\pm x_i, i \in S}}$).

\begin{algorithm}
\caption{Streaming $\linf$ Subspace Sketching\label{alg:subspace_sketching}}
\begin{algorithmic}[1]
    \STATE \textbf{Input}: A stream of points $x_1, \dots, x_n$, a value $r$ such that we have $r\cdot B_2^d \subseteq \conv{\inbraces{\pm x_1,\dots,\pm x_n}}$, and access to $\cU(\cE, x)$, the update rule for Algorithm \ref{alg:general_greedy_maxev} with state $\cE$, input $x$, and aspect ratio upper bound $\xi$.
    \STATE \textbf{Output}: Subset $S \subseteq [n]$ of size $O\inparen{d\logv{\nfrac{R}{r}+1}}$ for which $X\vert_S \subseteq X \subseteq O\inparen{\sqrt{d\logv{d\cdot\nfrac{R}{r}+1}}} \cdot X\vert_S$.
    \STATE Initialize $\cE_0 = 0$. Initialize $S = \emptyset$.
    \FOR{$t = 1, \ldots, n$}
        \STATE Read point $x_t$ from the stream.
        \IF{$\norm{x_t} > r$ and $x_t \notin \cE_{t-1}$}
            \STATE Let $\cE_t = \cU(\cE_{t-1}, e\cdot x_t, \xi)$.
            \STATE Update $S$: $S \gets S \cup \inbraces{t}$.
        \ELSE
            \STATE Let $\cE_t = \cE_{t-1}$.
        \ENDIF
    \ENDFOR
    \STATE \textbf{Output}: $S$.
\end{algorithmic}
\end{algorithm}

Algorithm \ref{alg:subspace_sketching} yields Theorem \ref{thm:subspace_sketching_ours}.

\begin{theorem}
\label{thm:subspace_sketching_ours}
Let $X \in \R^{n\times d}$ be presented in one pass over a row arrival stream. There is an algorithm $\cA$ which maintains a coreset $S \subseteq [n]$ such that:
\begin{align*}
    \text{for all } y \in \R^d, \maxnorm{X\vert_S \cdot y} \le \maxnorm{Xy} \le \alpha \cdot \maxnorm{X\vert_S \cdot y}
\end{align*}
where in the online coreset model, $\alpha = O\inparen{\sqrt{d\logv{d\cdot\nfrac{R}{r}+1}}}$ and $\abs{S} \le O\inparen{d \logv{d\cdot\nfrac{R}{r}+1}}$.
\end{theorem}
\begin{proof}
We first prove Lemma \ref{lemma:cvx_hull_coreset}.

\begin{lemma}
\label{lemma:cvx_hull_coreset}
The output $S$ of Algorithm \ref{alg:subspace_sketching} satisfies the following properties:
\begin{itemize}
    \item $S$ consists of at most $O\inparen{d\logv{\nfrac{R}{r}+1}}$ elements.
    \item $X\vert_S \subseteq X \subseteq O\inparen{\sqrt{d\logv{\nfrac{R}{r}+1}}} \cdot X\vert_S$.
\end{itemize}
\end{lemma}
\begin{proof}
For notational simplicity, write $s \coloneqq d\logv{\nfrac{R}{r}}$.

Observe that when we add elements to $S$, the volume of the state ellipsoid increases by a factor of at least $e$ in each iteration. Hence, over $\abs{S}$ iterations, we have:
\begin{align*}
    \frac{\mathsf{Vol}_d(\cE_n)}{\mathsf{Vol}_d(\cE_1)} \ge e^{\abs{S}}
\end{align*}
To get an upper bound on the left hand side, we prove the following claim.
\begin{claim}
For some constant $C$, in Algorithm \ref{alg:general_greedy_maxev}, we have:
\begin{align*}
    \frac{\mathsf{Vol}_d(\cE_n)}{\mathsf{Vol}_d(\cE_1)}\le C^{\nfrac{d}{2}}\cdot\logv{\xi+1}^{\nfrac{d}{2}} \cdot \xi^d \cdot \inparen{\frac{\max_{i\in[n]} \norm{x_i}}{\min_{i\in[n]} \norm{x_i}}}^d
\end{align*}
\end{claim}
\begin{proof}
Let $\astar = \nfrac{1}{R} \cdot I$. Observe that this is a valid choice of $\astar$ as used in the proofs of Theorems \ref{thm:simple_alg_arb_ellipsoid} and \ref{thm:greedy_approx}. Recall that we show that the $n$th iterate of Algorithm \ref{alg:general_greedy_maxev} satisfies, for some constant $C$:
\begin{align*}
    \fnorm{\astar\cdot A_n^{-1}}^2 = \sum_{i=1}^d \sigma_{i,n}^2 \le Cd\logv{\xi+1}
\end{align*}
By the AM-GM inequality, we have:
\begin{align*}
    \detv{\astar\cdot A_{n}^{-1}}^{\nfrac{2}{d}} = \inparen{\prod_{i=1}^d \sigma_{i,n}^2}^{\nfrac{1}{d}} \le \frac{\fnorm{\astar\cdot A_n^{-1}}^2}{d} = \frac{\sum_{i=1}^d \sigma_{i,n}^2}{d} \le C\logv{\xi+1}
\end{align*}
Furthermore, recall that our first iterate in Algorithm \ref{alg:general_greedy_maxev} satisfies:
\begin{align*}
    \detv{\astar\cdot A_{1}^{-1}} = \detv{\astar} \cdot \detv{A_{1}^{-1}} &= \frac{1}{R^d} \cdot \frac{\norm{x_1}^d}{\xi^{d-1}} \\
    &\ge \frac{1}{R^d} \cdot \inparen{\frac{\min_{i \in [n]} \norm{x_i}}{\xi}}^d \\
    &= \inparen{\frac{\min_{i\in[n]} \norm{x_i}}{\max_{i\in[n]} \norm{x_i}}}^d \cdot \frac{1}{\xi^d}
\end{align*}
We now write:
\begin{align*}
    \frac{\mathsf{Vol}_d(\cE_n)}{\mathsf{Vol}_d(\cE_1)} = \frac{\detv{A_n^{-1}}}{\detv{A_1^{-1}}} = \frac{\detv{\astar\cdot A_{n}^{-1}}}{\detv{\astar\cdot A_{1}^{-1}}} \le C^{\nfrac{d}{2}}\cdot\logv{\xi+1}^{\nfrac{d}{2}} \cdot \xi^d \cdot \inparen{\frac{\max_{i\in[n]} \norm{x_i}}{\min_{i\in[n]} \norm{x_i}}}^d
\end{align*}
\end{proof}
Putting everything together gives:
\begin{align*}
    e^{\abs{S}} \le \frac{\mathsf{Vol}_d(\cE_n)}{\mathsf{Vol}_d(\cE_1)}\le C^{\nfrac{d}{2}}\cdot\logv{\xi+1}^{\nfrac{d}{2}} \cdot \xi^d \cdot \inparen{\frac{\max_{i\in[n]} \norm{x_i}}{\min_{i\in[n]} \norm{x_i}}}^d
\end{align*}
which implies:
\begin{align*}
    \abs{S} &\le \frac{d}{2}\log C + \frac{d}{2}\log\logv{\xi+1} + d\logv{\xi} + d\logv{\frac{\max_{i\in[n]} \norm{x_i}}{\min_{i\in[n]} \norm{x_i}}}\\
    &\lesssim d\logv{\xi+1}+d\logv{\frac{\max_{i\in[n]} \norm{x_i}}{\min_{i\in[n]} \norm{x_i}}}
\end{align*}
as desired.

We now focus on proving $X \subseteq O\inparen{\sqrt{s}} \cdot X\vert_S$.

Notice that for all $i \in S$, we have $\norm{x_i} \ge r$ (since we initialize $\cE_0 = r\cdot B_2^d$). Hence, we have $\nfrac{r}{\sqrt{d}}\cdot B_2^d \subseteq X\vert_S$. It follows that $\nfrac{r}{\sqrt{d}}$ is a valid initialization for Algorithm \ref{alg:greedy_maxev} on the subset $e \cdot S$. Therefore, the output of Algorithm \ref{alg:greedy_maxev} on $e \cdot S$, which we will denote as $\cE_S$, satisfies:
\begin{align*}
    \frac{\cE_S}{O\inparen{\sqrt{d\logv{d\cdot\nfrac{R}{r}+1}}}} \subseteq e \cdot X\vert_S \subseteq \cE_S
\end{align*}
Next, observe that we only run the update rule for Algorithm \ref{alg:greedy_maxev} on the scaled elements in $S$ when we run Algorithm \ref{alg:subspace_sketching}. This is equivalent to running Algorithm \ref{alg:greedy_maxev} on the scaled elements in $S$, and since we initialize Algorithm \ref{alg:subspace_sketching} to $\cE_0 = \nfrac{r}{\sqrt{d}} \cdot B_2^d$, we have that $\cE_S$ is the final state ellipsoid of Algorithm \ref{alg:general_greedy_maxev}. This yields:
\begin{align*}
    X \subseteq \cE_S
\end{align*}
Putting our inclusions together gives:
\begin{align*}
    \frac{X}{O\inparen{\sqrt{d\logv{d\cdot\nfrac{R}{r}+1}}}} \subseteq \frac{\cE_S}{O\inparen{\sqrt{d\logv{d\cdot\nfrac{R}{r}+1}}}} \subseteq e \cdot X\vert_S
\end{align*}
In the end, we write:
\begin{align*}
    \frac{X}{O\inparen{\sqrt{d\logv{d\cdot\nfrac{R}{r}+1}}}} \subseteq e \cdot X\vert_S \subseteq X
\end{align*}
which is enough, as the factor of $e$ gets absorbed into the big-$O$ notation.
\end{proof}

We now show how Algorithm \ref{alg:subspace_sketching} and Lemma \ref{lemma:cvx_hull_coreset} together imply Theorem \ref{thm:subspace_sketching_ours}. Define:
\begin{align*}
    K\vert_S \coloneqq \inbraces{y \in \R^d \suchthat \maxnorm{X\vert_S\cdot y} \le 1}
\end{align*}
By the argument from Appendix \ref{section:mvie} we have:
\begin{align*}
    K\vert_S \subseteq K\vert_{[n]} \subseteq O\inparen{\sqrt{d\logv{d\cdot\nfrac{R}{r}+1}}}\cdot K\vert_S
\end{align*}
This is equivalent to:
\begin{align*}
    \text{for all } y \in \R^d, \maxnorm{X\vert_S \cdot y} \le \maxnorm{Xy} \le O\inparen{\sqrt{d\logv{d\cdot\nfrac{R}{r}+1}}} \cdot \maxnorm{X\vert_S \cdot y}
\end{align*}
as desired.
\end{proof}
